# Supplementary material for: Cavity-mediated long-range interactions in levitated optomechanics
Source: arXiv:2308.14721 source file (2023-08-28)
Supplement: Supplementary file 1 [file 6_2particle_Cooling.tex]

\centerline{\textbf{Two particle cavity cooling}}
\label{sec:cooling}
\vspace{1mm} 
By changing the RF frequencies applied to the AODs, we separate the laser frequencies $\omega_1$, $\omega_2 = \omega_1 - \delta$ by $\delta/2\pi = 300\,$kHz to eliminate any coherent scattering coupling. 
As $\delta<\kappa$ both particles can still couple to the same cavity mode individually and be cooled by coherent scattering, however with different detunings $\Delta_2 = \Delta_1 + \delta$. 
At a pressure of $10^{-6}\,$mbar we record spectra of the $y$ motion of particles $1$ and $2$ shown in Figure S~\ref{fig:cooling}a and b, respectively.
We employ sideband thermometry~\cite{Piotrowski2023} to measure occupation numbers of few hundreds from the fitted lines of the $y$-modes (see Figure S~\ref{fig:cooling}c).
The occupation numbers coincide for $\Delta_2 = \Delta_1$.
From the same fits we also get an estimate of the optomechanical couplings $g_\text{1}/2\pi\approx g_\text{2}/2\pi\approx 32\,$kHz consistent with the calculations from system parameters in the previous section.
\begin{figure}
    \centering
    \includegraphics[width = 9cm]{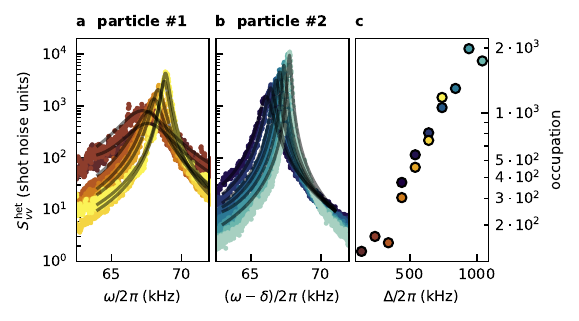}%{Figures/Figure2_v05.pdf}
    \caption{Figure S3. \textbf{Two particle cavity cooling.}
    % \textbf{A}.~The sketch depicts two particles held by tweezers with optical frequencies $\omega_\text{tw}$ placed within the TEM$_\text{00}$ mode of an optical cavity which is detuned with respect to the tweezers by $\Delta = \omega_\text{cav} - \omega_\text{tw}$.
    \textbf{a},~Power spectral densities for different detunings of particle 1 with trap frequency $\omega_1$
    \textbf{b},~Power spectral densities for different detunings of particle 2 with trap frequency $\omega_2=\omega_1+\delta$ with $\delta/2\pi = 300\,$kHz
    \textbf{c},~Occupation numbers extracted from fits in a,b.
    % Fitted splittings overlap with twice the coupling.
    }
    \label{fig:cooling}
\end{figure}

Investigating the interplay between cavity-mediated coupling and cooling will be an interesting next step, and is expected to have important consequences for optomechanics.
In particular, coherent scattering with coupled oscillators can be harnessed to cool collective mechanical modes, which has the potential to outperform current levitation-based sensing schemes and open up the study of emergent many-body effects in mesoscopic systems.

\vspace{5mm}
